# Supplementary material for: Disorder-induced gap in the normal density of states of the organic superconductor $\kappa$-(BEDT-TTF)$_2$Cu[N(CN)$_2$]Br
Source: arXiv:1410.5245 ancillary file (2014-10-20)
Supplement: Supplementary file 1 [file supplementary_arxiv.pdf]

# Temperature-dependent density of states in the organic superconductor $\kappa$-(BEDT-TTF)$_2$Cu[N(CN)$_2$]Br

Sandra Diehl,[1,2,*] Torsten Methfessel,[2] Jens Müller,[3] Michael Lang,[3] Michael Huth,[3] Martin Jourdan,[2] and Hans-Joachim Elmers[2]

[1]*Graduate School Materials Science in Mainz, Staudingerweg 9, 55128 Mainz, Germany*
[2]*Institut für Physik, Johannes Gutenberg-Universität Mainz, Staudingerweg 7, 55128 Mainz, Germany*
[3]*Physikalisches Institut, Goethe-Universität Mainz, Max-von-Laue-Str. 1, 60438 Frankfurt am Main, Germany*

(Dated: October 20, 2014)

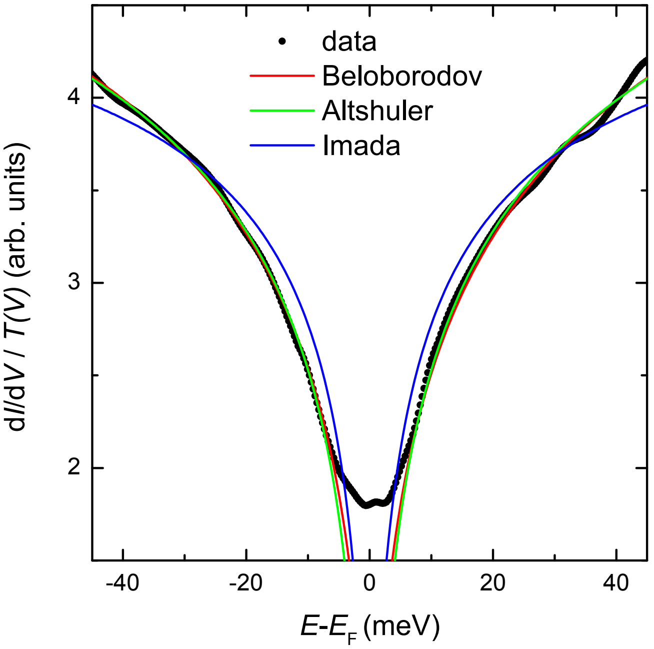


FIG. 1. Comparison of the models proposed by Beloborodov, Altshuler and Imada et al.. The model of Imada et al. (blue line) does not fit to the measured data. Whereas the model of Altshuler (green line) and Beloborodov (red line) describe the data qualitatively well. A quantitative description with reasonable fitting parameters is only possible with the model of Beloborodov et al. The fitting parameters obtained from the fit with Altshulers model deviate in orders of magnitude from values obtained by rough calculations.

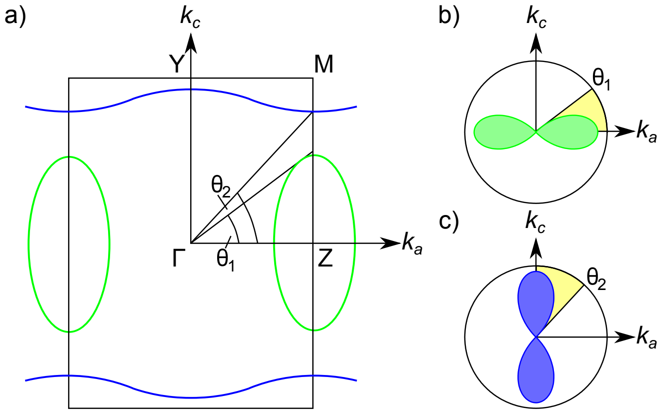


FIG. 2. a) Due to the twofold Fermi surface of the $\kappa$-Br crystals there are two different contributions to the measured superconducting gap function leading to two different values of the gap width $\Delta$. b),c) Therefore, it is necessary to use $\frac{c_1}{\theta_1}\int_0^{\theta_1} \mathrm{d}\theta \frac{E+i\Gamma}{\sqrt{(E+i\Gamma)^2-(\Delta_1\theta)^2}} + \frac{c_2}{\pi/2-\theta_2}\int_{\theta_2}^{\pi/2} \mathrm{d}\theta \frac{E+i\Gamma}{\sqrt{(E+i\Gamma)^2-(\Delta_2(\theta))^2}}$ for the determination of the two different values of the gap width.

TABLE I. Comparison of the different models.

| | |
|---|---|
| Beloborodov | $\gamma\left(1-\frac{1}{4\pi g_T^0}\ln\left(\frac{g_T^0 E_C}{\lvert eV\rvert}\right)\right)^{4g_T^0}$ |
| Althsuler | $\beta\left(1-\frac{\hbar}{2\pi E_{\mathrm{F}}\tau}\ln\left(\lvert E\rvert\frac{\tau}{\hbar}\right)\ln\left(\left\lvert\frac{E}{\hbar D\kappa^2}\right\rvert\right)\right)$ |
| Imada | $\alpha\exp(-\sqrt{(\epsilon_0/\epsilon)})$ |

TABLE II. Fit parameters of fit with the Dynes function.

| T (K) | $\Delta_1$ (meV) | $\Delta_2$ (meV) | $\Gamma$ (meV) |
|---|---|---|---|
| 5 | 2.80 | 6.4 | 1.80 |
| 7 | 2.40 | 5.4 | 1.45 |
| 9 | 2.05 | 4.8 | 1.35 |
| 11 | 1.35 | 3.2 | 0.80 |
